# Supplementary material for: R3-VAE: Reference Vector-Guided Rating Residual Quantization VAE for Generative Recommendation
Source: arXiv:2604.11440 source file (2026-05-06)
Supplement: Supplementary file 1 [file appendix.tex]

\section{Hello World}
%\subsection{Hello World}
